# Supplementary material for: Shift Graphs, Chromatic Number and Acyclic One-Path Orientations
Source: arXiv:2308.14010 source file (2024-12-17)
Supplement: Supplementary file 1 [file appendix.tex]

%------------------------------------------------------------------------------------------
\section{An example}
\label{app:tight-example}
%------------------------------------------------------------------------------------------
 shows that the \textsc{Directed-DomSet} has approximation 
ratio $\Omega(d^2)$. First, vertex $a_1$ arrives, which will be put  into $U$ and~$\Dalg$.
Then $a_2$ and $v_1,\ldots,v_{d^2}$ arrive, with an outgoing edge to~$a_1$. These
vertices are dominated by~$a_1$, so $U$ and $\Dalg$ are not modified.
Next, $w_1,\ldots,w_d$ arrive.
Vertex $w_1$ arrives with neighbors $v_1,\ldots,v_d$. We have $U=\Dalg=\{a_1\}$,
so $w_1$ is not dominated by any node in $\Dalg$ and it is not related to any node in $\Dalg$. 
Hence, $w_1$ will be put  into $U$ and~$\Dalg$. 
Then vertex $w_2$ arrives with neighbors $v_{d+1},\ldots,v_{2d}$. We have $U=\Dalg=\{a_1,w_1\}$,
so $w_1$ is not dominated by any node in $\Dalg$ and it is not related to any node in $\Dalg$. 
Hence, $w_2$ will be put  into $U$ and~$\Dalg$. Similarly, $w_3,\ldots,w_d$
will all be put into $U$ and $\Dalg$.
Then $x_1,\ldots,x_{d(d-1}$ arrive, each with one outgoing edge, to a unique node
among $v_1,\ldots,v_{d^2}$, as shown in the figure. They are all related to a node in $U$,
namely one of the $w_i$'s, so their out-neighbors will be out into $\Dalg$.
Finally, $z$ arrives, which is also put into $\Dalg$.
Hence, at the end of the algorithm $|\Dalg|=d^2+2$, but $\opt=3$ since $\{a_1,a_2,z\}$
is a dominating set.

%--------------------------------------------------------------------------------------

%--------------------------------------------------------------------------------------
